# Supplementary material for: GeneQuery: A General QA-based Framework for Spatial Gene Expression Predictions from Histology Images
Source: arXiv:2411.18391 source file (2024-11-27)
Supplement: Supplementary file 1 [file appendix.tex]

\section{Visualization of the Gene Embedding Space on HER2+}

\begin{figure*}[h]
\centering
\includegraphics[width=0.5\linewidth]{NeurIPS2024/figures/her2_gene_emb/her2_gene_DDT.pdf}
\caption{Visualization of the gene embedding space based on gene descriptions and the correlation between genes in the gene embedding space on the HER2+ dataset. Gray points represent all genes. The red point is the \textcolor{red}{anchor gene}, the blue point represents the gene with the \textcolor{blue}{highest correlation}, and the black point represents the gene with the \textbf{lowest correlation}.}
\label{fig:nameemb}
\end{figure*}

Figure~\ref{fig:nameemb} visualizes the learned gene embedding space based on gene description with t-SNE on the HER2+ datasets. 
The gray points refer to all gene description representations; 
the red point is the anchor gene DDT, a cancer-related gene. 
Results show that most gene spatial representations with higher Pearson correlation to the anchor point are also closer in space. 
This observation is consistent with that of GeneQuery on the GSE240429 data, indicating that GeneQuery has the potential to learn the relationships between different genes.

\newpage
\section{Gene Expression Pattern Visualization on HER2+}

\begin{figure*}[h]
\centering
\begin{tabular}{cc}
\subfigure[Observed Gene]{\includegraphics[width=0.25\linewidth]{NeurIPS2024/figures/her2_top/gold-s100A9.png}} 
\subfigure[STNet (R=0.1002)]{\includegraphics[width=0.25\linewidth]
{NeurIPS2024/figures/her2_top/stnet-S100A9}}
\subfigure[BLEEP (R=0.1191)]{\includegraphics[width=0.25\linewidth]{NeurIPS2024/figures/her2_top/bleep-S100A9.png}}
\subfigure[GeneQuery (R=0.1513)]{\includegraphics[width=0.25\linewidth]{NeurIPS2024/figures/her2_top/genequery-S100A9.png}} \\
\subfigure[Observed Gene]{\includegraphics[width=0.25\linewidth]{NeurIPS2024/figures/her2_top/gold-CLDN3.png}}
\subfigure[STNet (R=0.047)]{\includegraphics[width=0.25\linewidth]{NeurIPS2024/figures/her2_top/stnet-CLDN3.png}}
\subfigure[BLEEP (R=0.0595)]{\includegraphics[width=0.25\linewidth]{NeurIPS2024/figures/her2_top/bleep-CLDN3.png}} 
\subfigure[GeneQuery (R=0.1168)]{\includegraphics[width=0.25\linewidth]{NeurIPS2024/figures/her2_top/genequery-CLDN3.png}} \\
\subfigure[Observed Gene]{\includegraphics[width=0.25\linewidth]{NeurIPS2024/figures/her2_top/gold-DDT.png}}
\subfigure[STNet (R=0.0720)]{\includegraphics[width=0.25\linewidth]{NeurIPS2024/figures/her2_top/stnet-DDT.png}}
\subfigure[BLEEP (R=0.0060)]{\includegraphics[width=0.25\linewidth]{NeurIPS2024/figures/her2_top/bleep-DDT.png}} 
\subfigure[GeneQuery (R=0.1307)]{\includegraphics[width=0.25\linewidth]{NeurIPS2024/figures/her2_top/genequery-DDT.png}} \\
% \subfigure[gold-IGFBP2]{\includegraphics[width=0.25\linewidth]{NeurIPS2024/figures/her2_top/gold-IGFBP2.png}}
% \subfigure[STNet\_R=0.0587]{\includegraphics[width=0.25\linewidth]{NeurIPS2024/figures/her2_top/stnet-IGFBP2.png}}
% \subfigure[BLEEP\_R=0.1350]{\includegraphics[width=0.25\linewidth]{NeurIPS2024/figures/her2_top/bleep-IGFBP2.png}} 
% \subfigure[GeneQuery\_R=0.1307]{\includegraphics[width=0.25\linewidth]{NeurIPS2024/figures/her2_top/genequery-IGFBP2.png}} \\
\subfigure[Observed Gene]{\includegraphics[width=0.25\linewidth]{NeurIPS2024/figures/her2_top/gold-NAA10.png}}
\subfigure[STNet (R=0.0593)]{\includegraphics[width=0.25\linewidth]{NeurIPS2024/figures/her2_top/stnet-NAA10.png}}
\subfigure[BLEEP (R=0.0324)]{\includegraphics[width=0.25\linewidth]{NeurIPS2024/figures/her2_top/bleep-NAA10.png}} 
\subfigure[GeneQuery (R=0.1388)]{\includegraphics[width=0.25\linewidth]{NeurIPS2024/figures/her2_top/genequery-NAA10.png}} \\
\end{tabular}
\caption{Visualization of the gene expression pattern on the HER2+ dataset.}
\label{fig-her2_marker}
\end{figure*}

Figure~\ref{fig-her2_marker} shows four cancer-related genes, including S100A9, CLDN3, DDT, NAA10, on the HER2+ dataset. 
We compared GeneQuery with models that have comparable results, BLEEP and STNet. 
From the results, GeneQuery achieves a higher Pearson correlation for these genes and exhibits gene expression patterns more similar to the observed genes. 
The results are consistent with Figure ~\ref{fig:pear}.
